# Supplementary material for: Distributionally Robust Instrumental Variables Estimation
Source: arXiv:2410.15634 source file (2024-12-22)
Supplement: Supplementary file 1 [file additional-simulation.tex]

\begin{table}
\begin{centering}
\begin{tabular}{c|c|c|c|c|c|c}
$\eta$ & $\beta_{UZ}$ & OLS & TSLS & anchor & TSLS ridge & DRIVE\tabularnewline
\hline 
\hline 
0 & 0 & 1.12 & 1.39 & 1.12 & 1.12 & 1.39\tabularnewline
\hline 
0.4 & 0 & 1.12 & 14 & 1.11 & 1.12 & 0.56\tabularnewline
\hline 
0.4 & 0.4 & 1.21 & 7.2 & 1.20 & 1.21 & 0.98\tabularnewline
\hline 
0.4 & 0.8 & 1.17 & 2.50 & 1.17 & 1.17 & 1.39\tabularnewline
\hline 
0.8 & 0 & 1.14 & 40.42 & 1.13 & 1.14 & 0.14\tabularnewline
\hline 
0.8 & 0.4 & 1.26 & 21 & 1.30 & 1.26 & 1.18\tabularnewline
\hline 
0.8 & 0.8 & 1.37 & 11.89 & 1.34 & 1.37 & 1.48\tabularnewline
\end{tabular}
\par\end{centering}
\caption{Estimation errors of estimators when instruments are weak. Wasserstein
DRIVE performs well when there is direct effect from instruments to
the outcome and correlation with unobserved confounders is small. \zq{move to the appendix and add std information}}
\label{tab:weak-instrument}
\end{table}

\begin{figure}
\hspace*{-1.8cm} 
\begin{centering}
\includegraphics[scale=0.35]{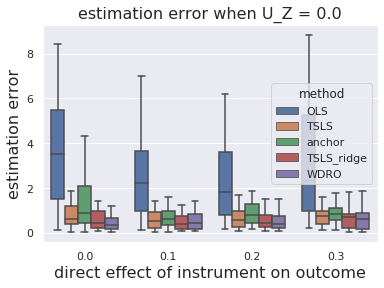}\includegraphics[scale=0.35]{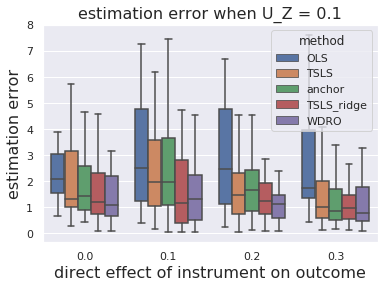}\includegraphics[scale=0.35]{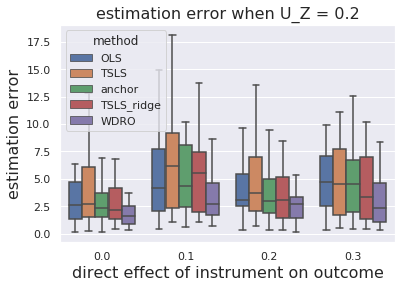}\includegraphics[scale=0.35]{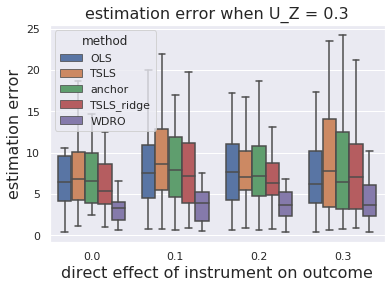}
\par\end{centering}
\caption{Estimation errors of different estimators when instruments are potentially invalid. Compared to \cref{fig:strongly-invalid-estimation-error}, the model used to generate this figure has milder instrument invalidity but stronger unobserved confounding. Wasserstein DRIVE (WDRO) consistently outperforms the other estimators. The $\ell^{2}$
norm of the true parameter is around $7$.}
\label{fig:mildly-invalid-estimation-error}
\end{figure}
